# Supplementary material for: Luminosity determination at HERA-B
Source: arXiv:0706.0131 source file (2007-06-01)
Supplement: Supplementary file 1 [file appendix.tex]

\subsection{Evidence for $\delta$ rays detection with the vertex detector}
\label{sec:delta}

When a proton of the beam crosses the wire target it has a certain
probability to produce delta-rays following the well known cross
section formula\cite{pdg}:
\begin{equation}\label{eq:delta}
\frac{{d^2 N}}{{dTdx}} = \frac{1}{2}Kz^2
\frac{Z}{A}\frac{1}{{\beta ^2 }}\frac{{F(T)}}{{T^2 }}
\end{equation}
where $N$ is the number of produced delta-rays,$T(MeV)$ is the
delta-rays kinetic energy, $x(\frac{g}{cm^2})$ is the thickness in
radiation length of the material crossed by the beam proton,
$K\sim0.307\; (MeV cm^2)$ is a constant, $z=1$ is the charge of
the proton beam, $Z$ and $A$ are the atomic number and weight of
the target material, $\beta$ is the velocity of the proton beam
(in our case $\beta\sim 1$) and $F(T)$ is a function of the
delta-rays kinetic energy whose value approaches the unity for
$T<<T_{max}$ the latter value being the maximum allowed kinetic
energy of the produced delta-rays which can be expressed, with
clear meaning of symbols as:
\begin{equation}\label{eq:tmax}
T_{\max }  = \frac{{2m_e c^2 \beta ^2 \gamma ^2 }}{{1 +
\frac{{2\gamma m_e }}{M} + \left( {\frac{{m_e }}{M}} \right)^2 }}
\end{equation}
In the HERA-$B$ experimental conditions $T_{max}\sim 423 \;(GeV)$.\\
It has to be noticed that one important feature of the mechanism
of delta-rays production is that the emission polar angle
$\vartheta$ with respect to the beam proton direction is highly
correlated with the kinetic energy of the produced electron, this
relation being expressed by:
\begin{equation}\label{eq:theta}
\cos (\vartheta ) = \frac{T}{p}\frac{{p_{\max } }}{{T_{\max } }}
\end{equation}
$p$ being the electron momentum.By using the values previously
defined the latter Equation can be used to express the electron
momentum as a function of the polar angle:

\begin{equation}\label{eq:delta-momentum}
p(MeV) = \frac{{1.022(MeV)}}{{\sin (\vartheta )\tan (\vartheta )}}
\end{equation}
The acceptance of the $VDS$ for reconstructing track segments
originating by the target spans, roughly, in the interval
$0.01<\vartheta<0.7\;(rad)$. As a consequence \hb is able to
reconstruct delta-rays produced in the momentum range
$1.88<p<10220\;(MeV)$ and the condition $T<<T_{max}$ is well
satisfied,
leading as a consequence, that we can consider $F(T)\sim 1$ in Equation~\ref{eq:delta}.\\
The limit on the average number of times that a single proton of
the beam can cross the target so producing delta-rays is set by a
total thickness of material equal, on average, to one interaction
length $\lambda _I$. In fact, when the proton undergoes an
interaction with a nucleus of the target, it can not produce
delta-rays any longer.Therefore, by using Equation\ref{eq:delta},
we can evaluate the average number of delta-rays produced per
interaction ($\left\langle {\frac{{N_\delta  }}{{IA}}}
\right\rangle$):
\begin{eqnarray}\label{eq:ndelta}
\left\langle {\frac{{N_\delta  }}{{IA}}} \right\rangle  & = &
0.154\frac{Z}{A}\int\limits_0^{\lambda _I } {dx}
\int\limits_{T_{\min } }^{T_{\max } } {\frac{1}{{T^2 }}} dT =
0.154\frac{Z}{A}\lambda _I \left( {\frac{1}{{T_{\min } }} -
\frac{1}{{T_{\max } }}} \right) \sim \nonumber \\ & \sim  &
0.154\frac{Z}{A}\frac{{\lambda _I }}{{T_{\min } }}
\end{eqnarray}
where the constant is calculated in such a way that $\lambda _I$
is in $\frac{g}{cm^2}$ and $T_{\min }$ is in $MeV$. This last
equation relates the total number of produced delta rays to the
total number of $pN$ interactions, so giving a possibility to
determine the luminosity for a data taking by counting the number
of reconstructed delta ray signals and correcting this number by
the reconstruction
efficiency ($\varepsilon_{\delta}$).\\
In order to calculate the term $\varepsilon_{\delta}$ implemented
a delta rays Monte Carlo generator in our full detector simulation
based on GEANT4. After some studies we concluded that a reasonable
value for the minimal kinetic energy $T_{\min }$, for the delta
rays event generation, was $1\;MeV$. We found typical values for
$\varepsilon_{\delta}$ of about 8\% for all the target materials
but this number is affected by an estimated systematic uncertainty
around 15\% substantially due to two main reasons (studied with
details):
\begin{itemize}
\item the distribution of the material between the wire target and
the $VDS$ system was good enough for describing tracks from $pN$
interactions characterized by high momentum ($>1\;GeV$), but quite
inaccurate for correctly describing low momentum (few $MeV$) delta
rays. \item The delta rays reconstruction efficiency depends also
critically by the simulation parameter defining the minimal
kinetic energy ($CUTELE$, in GEANT4) for which a track is followed
in the setup. This parameter, depending also from the threshold on
the $VDS$ signal amplitude to define a hit, was estimated around
$30\;keV$ for our detector. Unfortunately, the Monte Carlo
simulation showed that the $\varepsilon_{\delta}$ parameter starts
being critically dependent from $CUTELE$ for values right around
$30\;keV$.
\end{itemize}

The attempt to provide an independent and precise luminosity
determination using delta rays counting was therefore not possible
in our setup. We will describe now the experimental evidence we
collected for the detection of delta rays in our setup.\\
We will refer to some set of data completely acquired with pseudo
random trigger for the usual three types of wire material: Carbon,
Titanium and Tungsten. In the following we will report some
results using only the Carbon wire target, but anticipating that
similar
results were obtained also for the other two wire materials.\\
In order to select a sample of reconstructed delta rays we simply
selected events not passing the $IA$ trigger condition
\footnote{Although these data samples were acquired with pseudo
random trigger for each event the flag of the $IA$ trigger was
available.} and searched for segment of tracks reconstructed from
$VDS$. Note that this selection is optimal to select events in
which only few low momentum tracks are generated, like in the
delta rays
production case.\\
We then plotted the reconstructed $VDS$
  segments extrapolation to the Carbon target
  $Z$ position for the $X$ \footnote{In the following we will make use
of the definition of the orthogonal coordinate system for our
experiment:$Z$ coordinate in the beam axis direction, and $X$
("horizontal") and $Y$ ("vertical") defining a plane perpendicular
to it.The polar angle, $\theta$ is defined in such a way that
$\theta=0$ coincides with the $Z$ axis.} (and $Y$) coordinates.
The resulting distributions for $X$ and for events containing one
and two reconstructed $VDS$ segment is reported in
Figure~\ref{fig:delta_xdist}
\begin{figure}
  \centering
  \includegraphics*[bb=218 371 600 480,width=\textwidth]{figures/delta_xdist.eps}
  \caption{\it Reconstructed $VDS$
  segments extrapolation to the Carbon target
  $Z$ position for the $X$ coordinate (in $cm$)
  for events
  missed by the $IA$ trigger. In the left and right plots
  are reported, respectively, events with only one and two
  reconstructed $VDS$ segments. The target nominal position
  is not subtracted. A broad peak from low momentum tracks
  (attributed to delta rays) is clearly seen superimposed to a much
  narrower peak coming from high momentum tracks of normal
  $pN$ interactions. Similar plots were found for the $Y$
  coordinate.
   } \label{fig:delta_xdist}
\end{figure}

A broad peak from low momentum tracks (attributed to delta rays)
is clearly seen superimposed to a much narrower peak coming from
high momentum tracks of normal $pN$ interactions. By inspecting
these plots we were able to improve our selection of delta rays
tracks by adding a cut on $|Y|>1\; mm$ (so excluding high momentum
tracks from
normal $pN$ interactions).\\
The presence of low momentum tracks submitted to high Coulomb
scattering is anyway not enough to clearly claim the detection of
delta rays in our detector.\\
The main pieces of evidence we collected are instead summarized in
Figure~\ref{fig:delta_dist} in which we report a comparison
between real data (solid lines) and Monte Carlo
  (points with error bars) for different distributions relative to data
  taken with Carbon target. The Monte Carlo data were obtained by the
  delta rays events generator and the event selection was performed
  with the above mentioned criteria both on the real and Monte Carlo
  data samples.

\begin{figure}
  \centering
  \includegraphics*[bb=54 41 654 588,width=\textwidth]{figures/delta_dist.eps}
  \caption{\it Comparison between real data (solid lines) and Monte Carlo
  (points with error bars) for different distributions relative to data
  taken with Carbon target. The Monte Carlo
  normalization is on the total number
  of real data selected events.
   The event selection concerns events
  missed by the $IA$ trigger and containing only one reconstructed
  $VDS$ segment originating
  from  $|Y|>1\; mm$ (so excluding high momentum tracks from
  normal $pN$ interactions). A): distribution of the $VDS$ layer from
  which the reconstructed segments originate.
  The other three plots show quantities for
  segments originating from the first $VDS$ layer.
  B): polar angle $\theta$. C): impact
  point distributions in the $X$ and $Y$
  coordinates of the first $VDS$ layer. D): impact point
  distribution (in $X$ and $Y$) of the
  segment direction extrapolated to the target wire $Z$ position.
  The partial filling of the bins around $Y=0$ is just due to the
  binning.} \label{fig:delta_dist}
\end{figure}

In Figure~\ref{fig:delta_dist}A the distribution of the $VDS$
layer from which the reconstructed segments originate is reported.
The other three plots of Figure~\ref{fig:delta_dist} show some
other distributions for  segments originating from the first $VDS$
layer. In Figure~\ref{fig:delta_dist}B,
Figure~\ref{fig:delta_dist}C and Figure~\ref{fig:delta_dist}D the
polar angle $\theta$, impact
  point distributions in the $X$ and $Y$
  coordinates of the first $VDS$ layer and the impact point
  distribution (in $X$ and $Y$) of the
  segment direction extrapolated to the target wire $Z$ position
  are, respectively, reported.\\
 The agreement between real data and Monte Carlo simulation is, for
 all these distributions,
amazingly good, but the normalization is performed, for each of
them, on the total number of the real data selected events.\\
 As previously stated, an absolute normalization could not be achieved
with a systematic uncertainty better than 15\% or so.

%%%%%%%%%%%%%%%%%%%%%%%%%%%%%%%%%%%%%%%%%%%%%%%%%%%%%%%%%%%%%
\xx{
We have then evaluated $\left\langle {\frac{{N_\delta  }}{{IA}}} \right\rangle$ in two ways.\\
In the first method we just used Equation~\ref{eq:ndelta} by using
the relationship:
\begin{equation}\label{lambdai}
\lambda _I = \frac{A}{\sigma_{inel}N_A}
\end{equation}
where $N_A$ is the Avogadro's number and assuming
$T_{min}=1\;MeV$.
\begin{table}[h]
\centering
\includegraphics*[bb=96 345 589 477,width=\textwidth]{tables/ndelta.eps}
\caption{\it Average number of delta-rays produced per interaction
($\langle \frac{N_\delta}{IA} \rangle_A$) for different target
materials.The comparison between values using values in
References~\cite{joao}, \cite{pdg} (PDG) and the results with $MC$
$GEANT\;4$ simulation is presented.(The numbers for "GEANT 4" were
kindly provided by B. Schwingeneuer).The results of the ratios to
Carbon, $R_{AC}$ and their average,$\langle R_{AC} \rangle$,are
also reported. \label{table:ndelta}}
\end{table}
}
